# Supplementary material for: FreshMem: Brain-Inspired Frequency-Space Hybrid Memory for Streaming Video Understanding
Source: arXiv:2602.01683 source file (2026-10-08)
Supplement: Supplementary file 1 [file appendix2-new.pdf]

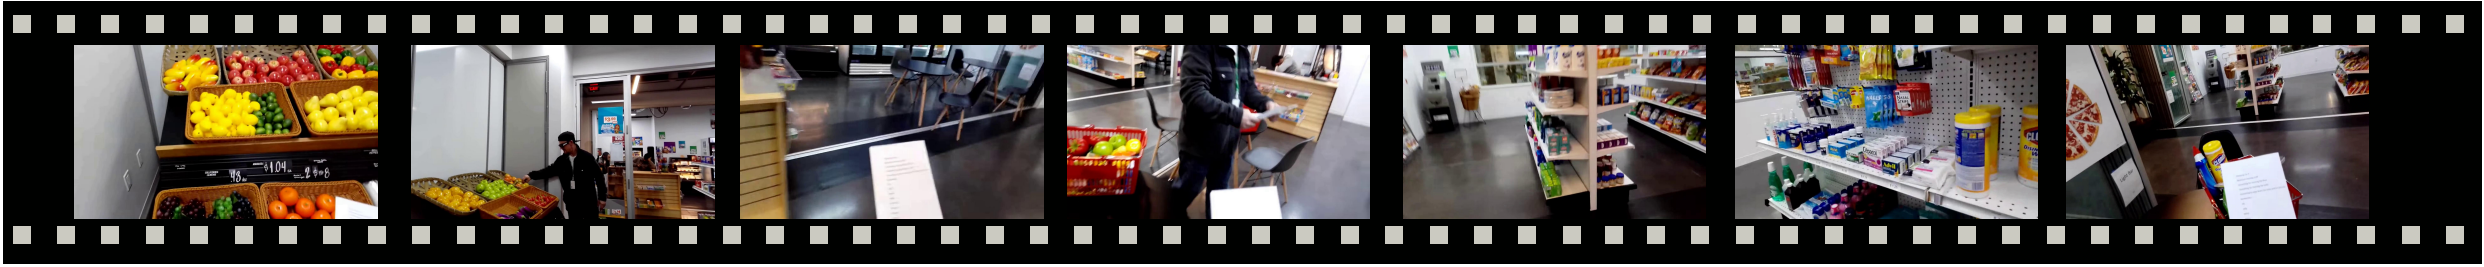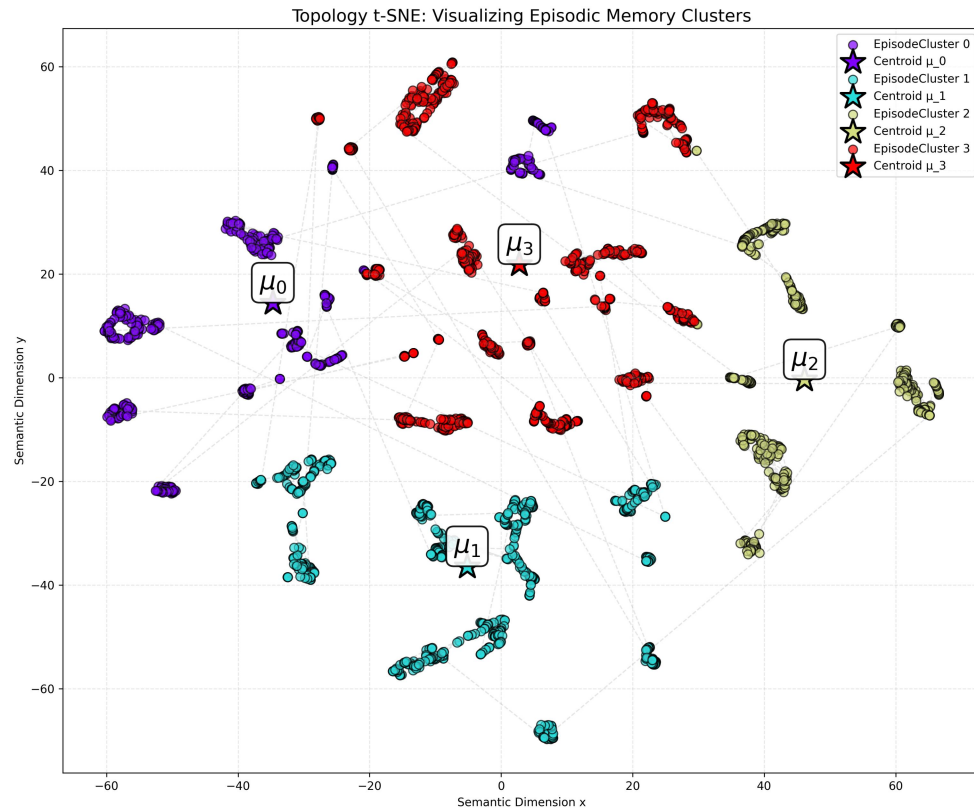

**Question:** Early in the video, while walking through the produce section, the camera captured a man wearing a black jacket and sunglasses. What specific color of apples was he reaching for?

**Options:**

**A:**Red

**B:**Green

**C:**Yellow

**D:**He was reaching for oranges

**Answer: B**

**Model Prediction: B**

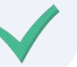

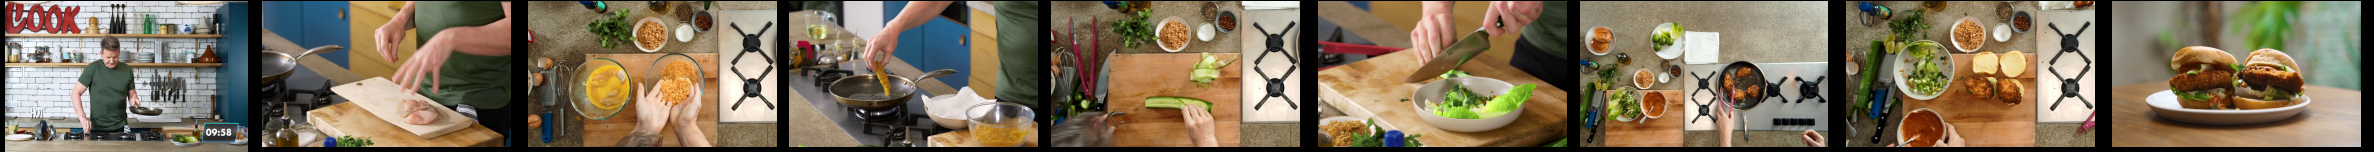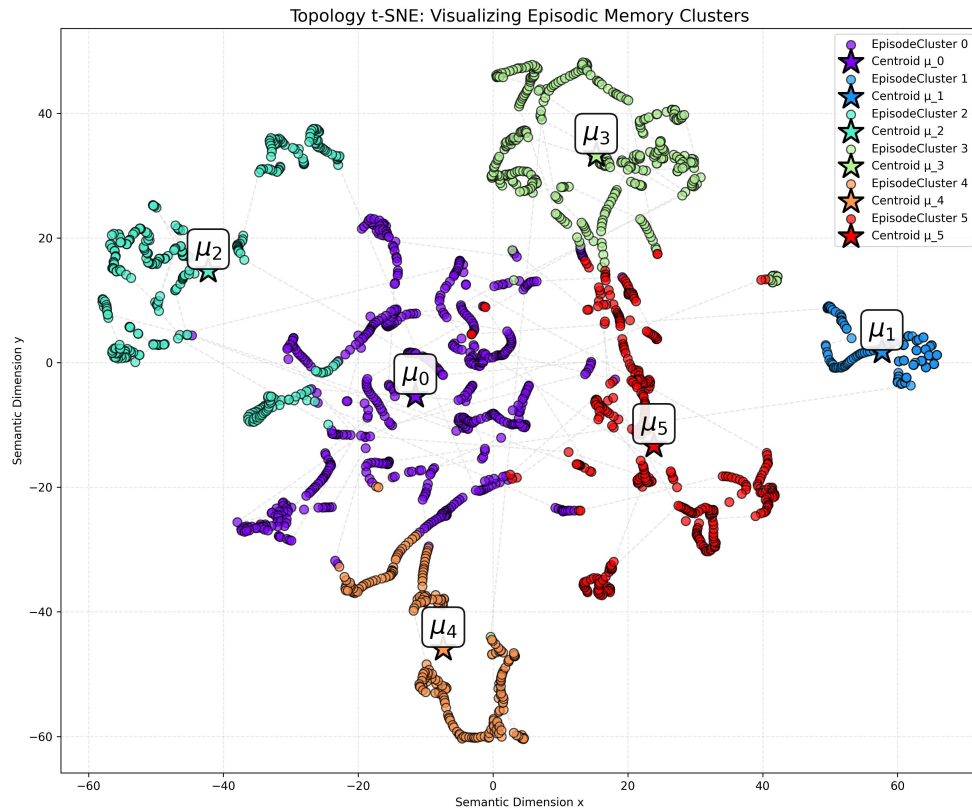

**Question:** During the frying and assembly stages, a specific pair of tongs is placed on the stovetop and later used to move ingredients. What is the color of these tongs?

**Options:**

A: Silver

B: Black

C: Magenta

D: Blue

**Answer: C**

**Model Prediction: C** ✓
